# Supplementary material for: Improving Deep Neural Network Random Initialization Through Neuronal Rewiring
Source: arXiv:2207.08148 source file (2022-07-17)
Supplement: Supplementary file 1 [file appendix.tex]

\clearpage
\appendix
\pagenumbering{gobble}
\setcounter{table}{0}

\section{Experiments with fully connected architectures}\label{appendix}

Additionally, we performed classification experiments with a simple model: a fully connected architecture with two hidden layers with 64 ReLU neurons each (referred to as shallow-thin). The intuition is to verify the effects of PA rewiring on a small scale with simple architectures. The model is trained on MNIST and FMNIST datasets, which are composed of grayscale images with simpler visual patterns. The experimental setup and performance evaluation are carried out considering the simple learning schedule and the statistical analysis described in the main paper.
% as in the paper?
The results for this architecture are shown in Table~\ref{tab:comparisons2}. It is possible to observe that PA rewiring improved the training metrics in the majority of cases, and improved final test accuracy for most cases on the MNIST dataset. On the FMNIST dataset, the same is observed regarding training performance, but not after training. In this case, although the proposed method improved training and convergence, in the end, the models reached a similar performance. This could be due to the limitation of this very small architecture for the given tasks.

\begin{table*}[!htb]
	\centering
	\caption{\label{tab:comparisons2}Comparison of the proposed PA rewiring method applied to several weight initializers for the shallow-thin FC architecture. For each case, 100 models were trained, and colors represent the result of statistical tests performed between the base weights and the rewired version.}
	
	\begin{tabular}{cc|ccc|cc}
		\hline
    % 	&&\multicolumn{3}{c|}{convergence (epochs)} &\multicolumn{3}{c}{test accuracy ($\%$)} \\
    % 	& method &min&average&max&min&average& max \\
		& & \multicolumn{3}{c|}{training metrics} & \multicolumn{2}{c}{test acc.}  \\
		
		dataset&weights&ep.\ 1 acc.\ &ep.\ 1 val. acc.\ &convergence&average& median\\ 
		\hline \hline    
\multirow{8}{*}{\rotatebox[origin=c]{90}{MNIST}}
& Kaiming-Uniform&93.05{\tiny$\pm$0.36}&92.29{\tiny$\pm$0.44}&15.83{\tiny$\pm$4.14}&97.43{\tiny$\pm$0.12}&97.44{\tiny$\pm$0.12} \\
& PA rewiring&\cellcolor{green!45}93.38{\tiny$\pm$0.30}&\cellcolor{green!45}92.56{\tiny$\pm$0.34}&\cellcolor{gray!65}15.24{\tiny$\pm$4.00}&\cellcolor{green!45}97.47{\tiny$\pm$0.13}&\cellcolor{gray!65}97.47{\tiny$\pm$0.08} \\
& Kaiming-Normal&93.05{\tiny$\pm$0.32}&92.30{\tiny$\pm$0.35}&15.54{\tiny$\pm$3.63}&97.41{\tiny$\pm$0.13}&97.40{\tiny$\pm$0.13} \\
& PA rewiring&\cellcolor{green!45}93.27{\tiny$\pm$0.42}&\cellcolor{green!45}92.48{\tiny$\pm$0.44}&\cellcolor{gray!65}15.08{\tiny$\pm$2.99}&\cellcolor{green!45}97.45{\tiny$\pm$0.11}&\cellcolor{green!45}97.44{\tiny$\pm$0.07} \\
& truncated-normal&92.99{\tiny$\pm$0.41}&92.26{\tiny$\pm$0.41}&15.91{\tiny$\pm$3.79}&97.42{\tiny$\pm$0.11}&97.42{\tiny$\pm$0.11} \\
& PA rewiring&\cellcolor{green!45}93.33{\tiny$\pm$0.33}&\cellcolor{green!45}92.57{\tiny$\pm$0.34}&\cellcolor{gray!65}15.62{\tiny$\pm$4.40}&\cellcolor{green!45}97.47{\tiny$\pm$0.12}&\cellcolor{green!45}97.47{\tiny$\pm$0.08} \\
& Orthogonal&92.34{\tiny$\pm$0.38}&91.70{\tiny$\pm$0.42}&18.44{\tiny$\pm$5.17}&97.58{\tiny$\pm$0.11}&97.60{\tiny$\pm$0.11} \\
& PA rewiring&\cellcolor{green!45}92.61{\tiny$\pm$0.34}&\cellcolor{green!45}91.95{\tiny$\pm$0.36}&\cellcolor{gray!65}19.54{\tiny$\pm$5.13}&\cellcolor{gray!65}97.59{\tiny$\pm$0.13}&\cellcolor{gray!65}97.60{\tiny$\pm$0.09} \\
\hline
\multirow{8}{*}{\rotatebox[origin=c]{90}{FMNIST}}
& Kaiming-Uniform&83.31{\tiny$\pm$0.71}&82.81{\tiny$\pm$0.75}&26.34{\tiny$\pm$6.26}&88.28{\tiny$\pm$0.24}&88.27{\tiny$\pm$0.24} \\
& PA rewiring&\cellcolor{green!45}83.60{\tiny$\pm$0.65}&\cellcolor{green!45}83.03{\tiny$\pm$0.64}&\cellcolor{green!45}24.24{\tiny$\pm$7.70}&\cellcolor{gray!65}88.32{\tiny$\pm$0.24}&\cellcolor{gray!65}88.32{\tiny$\pm$0.16} \\
& Kaiming-Normal&83.18{\tiny$\pm$0.75}&82.80{\tiny$\pm$0.78}&25.44{\tiny$\pm$7.21}&88.19{\tiny$\pm$0.22}&88.22{\tiny$\pm$0.22} \\
& PA rewiring&\cellcolor{green!45}83.41{\tiny$\pm$0.75}&\cellcolor{green!45}83.02{\tiny$\pm$0.77}&\cellcolor{gray!65}25.02{\tiny$\pm$7.31}&\cellcolor{gray!65}88.22{\tiny$\pm$0.24}&\cellcolor{gray!65}88.23{\tiny$\pm$0.15} \\
& truncated-normal&83.22{\tiny$\pm$0.73}&82.84{\tiny$\pm$0.75}&26.13{\tiny$\pm$6.50}&88.22{\tiny$\pm$0.20}&88.22{\tiny$\pm$0.20} \\
& PA rewiring&\cellcolor{green!45}83.46{\tiny$\pm$0.64}&\cellcolor{gray!65}83.00{\tiny$\pm$0.65}&\cellcolor{green!45}24.08{\tiny$\pm$7.60}&\cellcolor{gray!65}88.24{\tiny$\pm$0.20}&\cellcolor{gray!65}88.24{\tiny$\pm$0.13} \\
& Orthogonal&82.77{\tiny$\pm$0.77}&82.48{\tiny$\pm$0.80}&29.14{\tiny$\pm$2.76}&88.43{\tiny$\pm$0.18}&88.46{\tiny$\pm$0.18} \\
& PA rewiring&\cellcolor{gray!65}82.94{\tiny$\pm$0.78}&\cellcolor{gray!65}82.66{\tiny$\pm$0.81}&\cellcolor{gray!65}29.25{\tiny$\pm$2.90}&\cellcolor{gray!65}88.43{\tiny$\pm$0.18}&\cellcolor{gray!65}88.42{\tiny$\pm$0.13} \\
\hline

	\end{tabular}
\end{table*}

We consider another FC architecture with increased complexity: eight hidden layers with 2048 ReLU neurons each (deep-wide). Compared to the shallow-thin architecture, this is another extreme case with traditional MLP-like models and the goal is to check the performance of the proposed method in such a scenario. The results are shown in Table~\ref{tab:comparisons3}, indicating a similar behavior as observed with the shallow-thin model. Training performance and convergence are improved in most of the cases, and test performance gains were observed when using the Kaiming-Uniform initializer. On the other hand, PA rewiring decreased the final test performance when using the Kaiming-Normal initializer on the MNIST dataset, even though it improved training for this particular case.

\begin{table*}[!htb]
	\centering
	\caption{\label{tab:comparisons3}Comparison of the proposed PA rewiring method with different weight initializers for the deep-wide FC architecture, trained on the MNIST and FMNIST datasets.}
	
	\begin{tabular}{cc|ccc|cc}
		\hline
    % 	&&\multicolumn{3}{c|}{convergence (epochs)} &\multicolumn{3}{c}{test accuracy ($\%$)} \\
    % 	& method &min&average&max&min&average& max \\
		& & \multicolumn{3}{c|}{training metrics} & \multicolumn{2}{c}{test acc.\ }  \\
		
		dataset&weights& ep.\ 1 acc.\ & ep.\ 1 val.\ acc.\ &convergence&average&median\\ 
		\hline \hline
\multirow{8}{*}{\rotatebox[origin=c]{90}{MNIST}}
& Kaiming-Uniform&95.74{\tiny$\pm$0.69}&94.47{\tiny$\pm$0.71}&5.94{\tiny$\pm$1.05}&98.10{\tiny$\pm$0.07}&98.10{\tiny$\pm$0.07} \\
& PA rewiring&\cellcolor{gray!65}95.92{\tiny$\pm$0.72}&\cellcolor{gray!65}94.49{\tiny$\pm$0.73}&\cellcolor{gray!65}5.66{\tiny$\pm$1.34}&\cellcolor{green!45}98.14{\tiny$\pm$0.08}&\cellcolor{green!45}98.14{\tiny$\pm$0.05} \\
& Kaiming-Normal&93.04{\tiny$\pm$2.52}&92.03{\tiny$\pm$2.40}&8.22{\tiny$\pm$2.82}&98.14{\tiny$\pm$0.10}&98.15{\tiny$\pm$0.10} \\
& PA rewiring&\cellcolor{green!45}95.96{\tiny$\pm$0.79}&\cellcolor{green!45}94.54{\tiny$\pm$0.77}&\cellcolor{green!45}5.55{\tiny$\pm$1.06}&\cellcolor{red!45}98.10{\tiny$\pm$0.08}&\cellcolor{red!45}98.11{\tiny$\pm$0.05} \\
& truncated-normal&95.75{\tiny$\pm$0.72}&94.46{\tiny$\pm$0.72}&5.79{\tiny$\pm$0.90}&98.12{\tiny$\pm$0.10}&98.12{\tiny$\pm$0.10} \\
& PA rewiring&\cellcolor{green!45}96.01{\tiny$\pm$0.81}&\cellcolor{gray!65}94.62{\tiny$\pm$0.81}&5.79{\tiny$\pm$1.26}&\cellcolor{gray!65}98.10{\tiny$\pm$0.08}&\cellcolor{gray!65}98.10{\tiny$\pm$0.05} \\
& Orthogonal&93.62{\tiny$\pm$0.69}&92.80{\tiny$\pm$0.71}&7.44{\tiny$\pm$1.07}&98.32{\tiny$\pm$0.06}&98.32{\tiny$\pm$0.06} \\
& PA rewiring&\cellcolor{green!45}93.83{\tiny$\pm$0.81}&\cellcolor{gray!65}92.98{\tiny$\pm$0.83}&\cellcolor{gray!65}7.48{\tiny$\pm$1.37}&\cellcolor{gray!65}98.32{\tiny$\pm$0.08}&\cellcolor{gray!65}98.33{\tiny$\pm$0.05} \\
\hline
\multirow{8}{*}{\rotatebox[origin=c]{90}{FMNIST}}
& Kaiming-Uniform&85.40{\tiny$\pm$1.09}&84.32{\tiny$\pm$1.04}&7.47{\tiny$\pm$0.84}&89.80{\tiny$\pm$0.21}&89.79{\tiny$\pm$0.21} \\
& PA rewiring&\cellcolor{green!45}86.14{\tiny$\pm$0.94}&\cellcolor{green!45}84.76{\tiny$\pm$0.92}&\cellcolor{green!45}6.84{\tiny$\pm$0.87}&\cellcolor{green!45}89.88{\tiny$\pm$0.25}&\cellcolor{green!45}89.90{\tiny$\pm$0.16} \\
& Kaiming-Normal&85.37{\tiny$\pm$1.04}&84.41{\tiny$\pm$1.03}&7.29{\tiny$\pm$0.86}&89.76{\tiny$\pm$0.20}&89.76{\tiny$\pm$0.20} \\
& PA rewiring&\cellcolor{green!45}86.13{\tiny$\pm$1.03}&\cellcolor{green!45}84.78{\tiny$\pm$0.98}&\cellcolor{green!45}6.92{\tiny$\pm$0.91}&\cellcolor{gray!65}89.75{\tiny$\pm$0.18}&\cellcolor{gray!65}89.76{\tiny$\pm$0.11} \\
& truncated-normal&85.51{\tiny$\pm$1.09}&84.48{\tiny$\pm$1.03}&7.26{\tiny$\pm$0.81}&89.79{\tiny$\pm$0.22}&89.80{\tiny$\pm$0.22} \\
& PA rewiring&\cellcolor{green!45}86.09{\tiny$\pm$0.95}&\cellcolor{green!45}84.79{\tiny$\pm$0.90}&\cellcolor{green!45}6.89{\tiny$\pm$0.85}&\cellcolor{gray!65}89.80{\tiny$\pm$0.21}&\cellcolor{gray!65}89.82{\tiny$\pm$0.15} \\
& Orthogonal&82.95{\tiny$\pm$1.18}&82.51{\tiny$\pm$1.20}&10.15{\tiny$\pm$1.18}&90.03{\tiny$\pm$0.18}&90.05{\tiny$\pm$0.18} \\
& PA rewiring&\cellcolor{gray!65}83.18{\tiny$\pm$1.31}&\cellcolor{gray!65}82.71{\tiny$\pm$1.30}&\cellcolor{green!45}9.82{\tiny$\pm$1.08}&\cellcolor{gray!65}90.08{\tiny$\pm$0.20}&\cellcolor{gray!65}90.08{\tiny$\pm$0.14} \\
\hline

	\end{tabular}
\end{table*}

The performance difference between the shallow-thin and deep-wide architectures shows that scaling a traditional FC model, in a traditional training schedule, results in a poor performance improvement for vision tasks. Nevertheless, we evaluated the PA rewiring method in such a scenario. The results show that the training performance is improved in most cases. As for the testing performance, the method usually improves performance or keeps it similar to that of the base weights, except for a single case with the deep-wide architecture.
